# Supplementary material for: Iterative map-making with two-level preconditioning for polarized Cosmic Microwave Background data sets
Source: arXiv:1801.08937 source file (2018-05-03)
Supplement: Supplementary file 1 [file arnoldi_appendix.tex]

\section{The Arnoldi Algorithm}
\label{subsec:arnoldi}

The \emph{Krylov } subspace algorithms are based upon the structure of a sequence of vectors naturally produced by the power method,  a class of  those, namely the  Minimal Residuals (MINRES) and the Generalized Minimal Residual (GMRES) methods \citep{Golub:1996:MC:248979} rely on the Arnoldi algorithm. 
\begin{figure}[!htbp]
\includegraphics[width=1.\columnwidth]{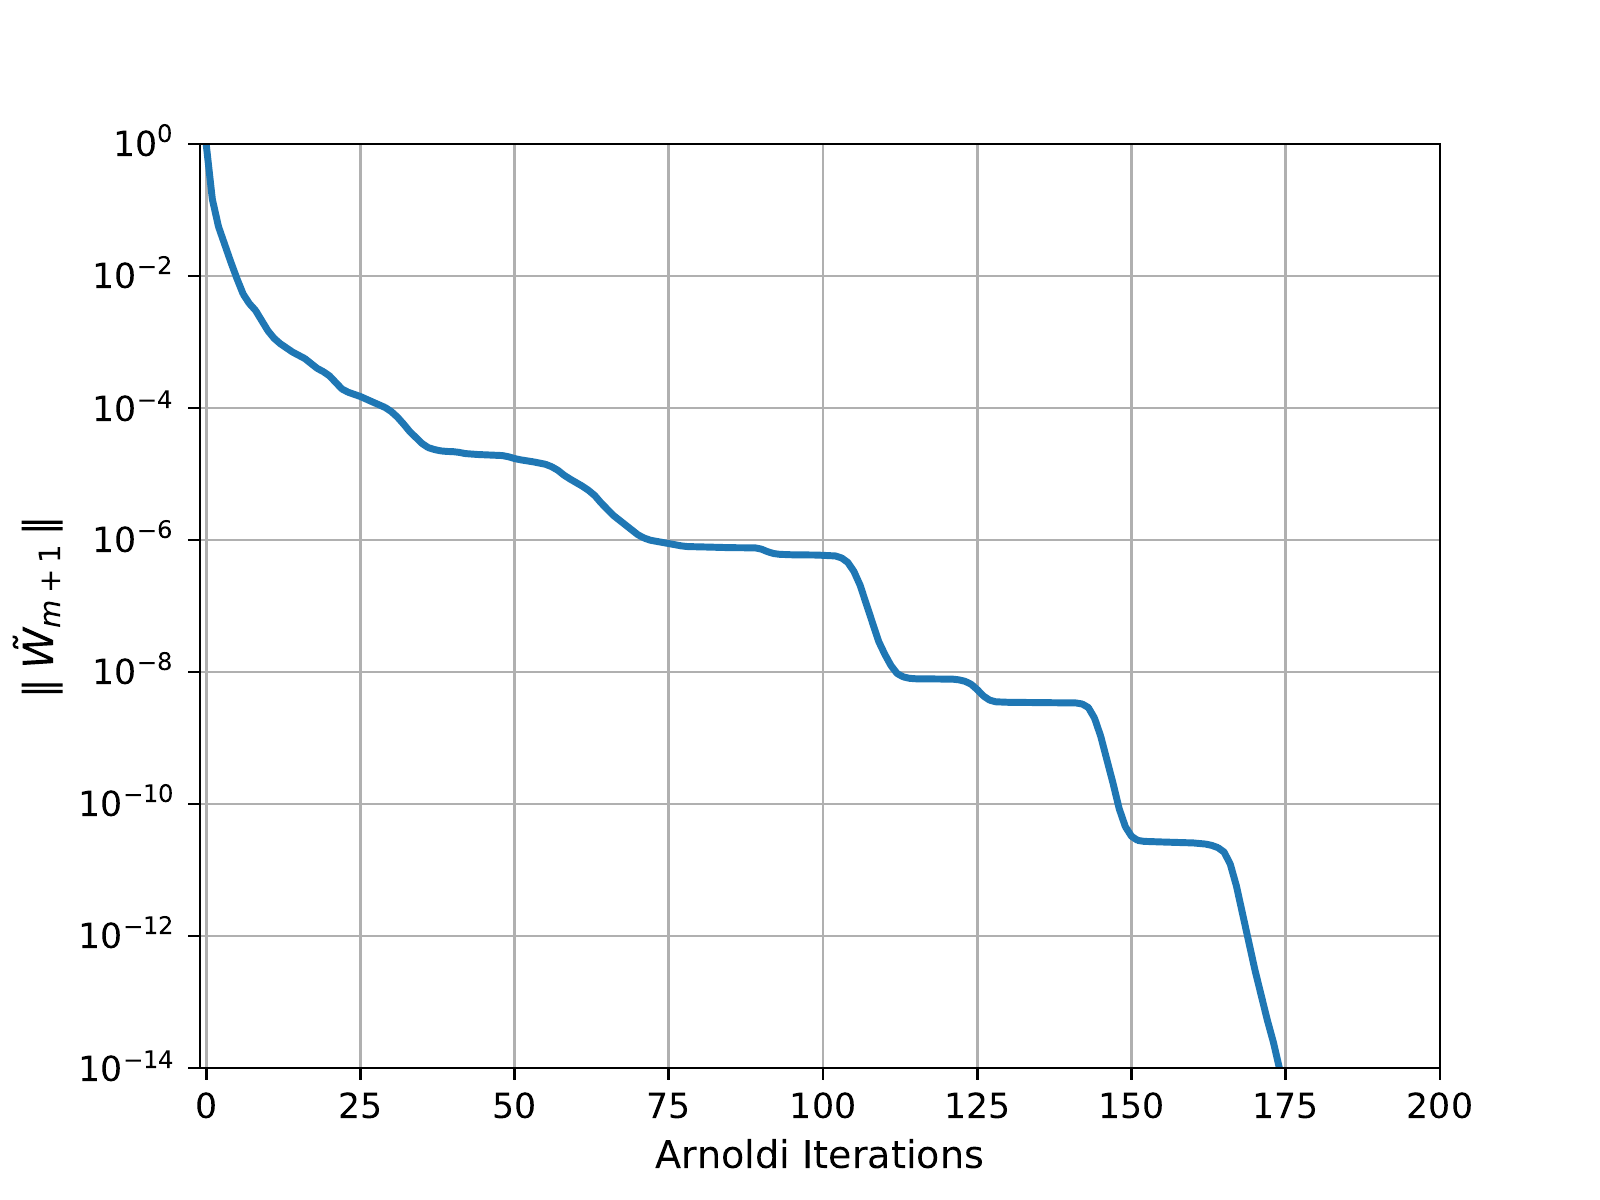}
\caption{The convergence residuals of the Arnoldi algorithm. Notice that after about $175 $ iterations the algorithm numerically converges.}\label{fig:arnoldires}
\end{figure}

Our aim is to find an approximation to the eigenvalues of a matrix $B$ of  a generic linear system with r.h.s.  $b$:
\begin{equation}
Bx=b.
\label{eq:newlinsys}
\end{equation}
The Arnoldi algorithm is an algorithm aimed at solving a linear system by projecting the system matrix onto a convenient  Krylov subspace generated by the first $m$ vectors: 
\begin{equation}
\mathcal{K}_m (B, b)= span \lbrace b, Bb,B^2 b, \dots, B^{m-1} b \rbrace,
\label{eq:krylov}
\end{equation}
and the algorithm steps are summarized in Algorithm \ref{alg:arnoldi}.
\begin{algorithm}[H]
\caption{Basic Arnoldi  Algorithm}\label{alg:arnoldi}
  \begin{algorithmic}[1]
    \Require : $r_0,\, w_1= r_0/\parallel r_0 \parallel$
    \For{j = 1$\rightarrow $ m}
    	\State $v_j=B w_j$
    \For{i = 1$\rightarrow $ j}
      \State $h_{i,j}= (v_j , w_i)$
    \EndFor
	\State    $v_j = v_j - \sum_{i=1} ^j h_{i,j} w_i$ 
	\State $h_{j+1,j} = \parallel  v_j\parallel$
	\If{$h_{j+1,j}\leq \mathrm{tol}_{Arn}$  }
		\State break
	\Else 
		\State $w_{j+1} = v_j / h_{j+1,j}$
	\EndIf
	\EndFor
  \end{algorithmic}
\end{algorithm}

Hence, the output of the Arnoldi algorithm is an orthonormal basis $W^{(m)}= (w_1| w_2|\dots| w_m)$ (called the \emph{Arnoldi vectors }), together with a set of scalars $h_{i,j}$ (with $i,j=1,\dots,m$ and $i\leq j+1$) plus an extra-coefficient $h_{m+1,m}$. The former set of coefficients are the elements of an upper Hessenberg matrix $H_m $ with non-negative subdiagonal elements and is commonly referred as a \emph{m-step Arnoldi Factorization} of $B$. If $B$ is Hermitian then $H_m$ is symmetric, real  and  tridiagonal and the vectors (columns of $W^{(m)}$) of the Arnoldi basis  are called \emph{Lanczos vectors}. $B$ and $H_m$ are intimately related via:
\begin{equation}
BW^{(m)} = W^{(m)} H _m + h_{m+1,m} w_{m+1} e^\dag  _m,
\label{eq:factoriz}
\end{equation}
where $e_m$ is a $1\times m $ unit vector with 1 on the $m$-th component.

 In other words, $H_m$ is the projection of $B$ onto the subspace generated by the Arnoldi basis $W^{(m)}$  within an error  given by $\tilde{W}_m= h_{m+1,m} w_{m+1} e^\dag  _m$.  The  iteration loop ends when this error term gets smaller than a  certain threshold $\epsilon_{tol}$.

Eq.~\eqref{eq:factoriz} is remarkable, since connects the eigenpairs of $B$ to the ones of $H_m$.
Let us consider an eigenpair of $H_m, \,(\lambda_i,y_i)$:
\begin{displaymath}
H_m y_i = \lambda_i y_i,
\end{displaymath}
then the vector $v_i= W^{(m)} y_i$ satisfies
\begin{equation}	
\parallel B v_i - \lambda_i v_i \parallel= \parallel ( B W^{(m)} - W^{(m)} H_m ) v_i \parallel=  \parallel \tilde{W}_m v_i \parallel.
\label{eq:ritz}
\end{equation}
\Ie\ the eigenpairs of $H_m$ are approximations  of the eigenpairs of $B$ within an  error given by $\tilde{W}_{m+1}$. They are the so called Ritz eigenpairs  and they are very easy to compute since the size of $H_m$ is  $\lesssim \mathcal{O}(100)$. For a typical \cmb dataset this is the order of Arnoldi iterations required to encompass a tolerance $tol_{Arn}\sim 10^{-6}$ as it is shown in fig.\ref{fig:arnoldires}.  

\begin{figure*}[!htb]
\includegraphics[width=2\columnwidth , clip=true, trim=0 6cm 0 0]{figures/ritz_eigenvalues_h.png}
\caption{Histograms of Ritz eigenvalues of the matrix $\mbd A$ computed for several choices of Arnoldi tolerance, $\epsilon_{Arn}$. }
\label{fig:binned_ritz}
\end{figure*}

\section{Dealing with non-orthogonal filters}
\label{app:filters}

As discussed in Sect. \ref{subsec:datamodel}, the ground and polynomial filtering are sequentially applied to the data, \ie\
\begin{displaymath}
F_T \equiv F_G F_B
\end{displaymath}
However, since we did not orthogonalize $F_T$ the system matrix $P^{\dag} F_T P$ is not symmetric and PCG convergence is not anymore ensured. 

To overcome this issue we exploit the properties of the filters following the definition in Eq.~\eqref{eq:filt}
\begin{align*}
F_B^{\dag} =F_B, \,&   F_G^{\dag} =F_G, \\
&\mbox{and}  \\
F_T^{\dag}  F_T= F_B F_G &F_G F_B= F_B F_G F_B\\ 
\end{align*}
where  for the first equality we make use of the definition in \ref{eq:filt} for $F_B $ and $F_G$ and for the last equality we exploited the property of idempotence of $F_G$, (being all the filter operators  defined in \ref{eq:filt}  \emph{projectors}). 
The two filters are then combined in such a way that the system matrix of the unbiased estimator is symmetric, \ie\
\begin{equation}
(F_T P)^{\dag}   F_T P= P^{\dag}    F_T^{\dag}  F_T P \equiv  P^{\dag}  F_B F_G F_B P = P^{\dag}  \tilde{F}_T P  \label{eq:systmatr}
\end{equation}
where $\tilde{F}_T = F_B F_G F_B$, is the \emph{Stompor} matrix and it  encodes all the filtering and weighting operations when applied to a time-domain vector and we use $P^{\dag} \tilde{F}_T P $ as a system matrix.
